# Supplementary material for: Frustration of the isotropic-columnar phase transition of colloidal hard platelets by a transient cubatic phase
Source: arXiv:1112.1209 ancillary file (2011-12-06)
Supplement: Supplementary file 1 [file suppinfo.pdf]

# Frustration of the isotropic-columnar phase transition of colloidal hard platelets by a transient cubatic phase: Supplementary Material

Matthieu Marechal,[*] Alessandro Patti,[†] Matthew Dennison, and Marjolein Dijkstra

*Soft Condensed Matter, Debye Institute for NanoMaterials Science, Utrecht University, Princetonplein 5, 3561 RT Utrecht, The Netherlands*

(Dated: December 2, 2011)

## Cluster criterion

The cluster criterion consists of the following steps: First, we define the neighbors of particle $i$ as those particles $j$ for which the surface-to-surface distance $\rho_{ij}$ is smaller than $0.2D$ and $\mathbf{u}_i \cdot \mathbf{u}_j > 0.9$ with $\mathbf{u}_i$ the orientation of particle $i$. We also define the set of particles $\mathcal{E}_i$ which contains $i$ and its neighbors and we define the plane $\mathcal{P}_i$ perpendicular to the nematic director $\mathbf{n}_i$ of the particles in $\mathcal{E}_i$. Then, we examine the trigonal, square and hexagonal order around particle $i$ in the plane $\mathcal{P}_i$,

$$\psi_n(i) = \left| \frac{1}{N_b(i)} \sum_{j=1}^{N_b(i)} \exp(\,\mathrm{i}\, n\phi_{ij}) \right| , \tag{1}$$

where $n = 3, 4, 6$, and $\phi_{ij}$ is the angle between $\mathbf{r}_{ij}^{\mathrm{proj}}$ and a reference axis, which lies in $\mathcal{P}_i$. Also, $\mathbf{r}_{ij}^{\mathrm{proj}}$ is the projection on $\mathcal{P}_i$ of the bond between particle $i$ and $j$. The sum over $j$ runs over the $N_b(i)$ neighbors of particle $i$ which are not in the same stack as $i$ (the values for $\phi_{ij}$ for $j$ in the same stack as $i$ are random for both isotropic and columnar phases). Furthermore, particles $i$ and $j$ are defined to be in the same stack if they are neighbors and their center-to-center distance $r_{ij}$ is smaller than $L + 0.2D$. We then make a distinction between particles with a columnar-like and an isotropic-like environment. Particle $i$ has a columnar-like environment if $\psi_6(i) > 0.6$ and $\psi_n(i) < 0.7$ for $n = 3, 4$. We define $n_{\mathrm{col}}(i)$ to be the number of particles in $\mathcal{E}_i$ that have a columnar-like environment. Those particles $i$ that have $n_{\mathrm{col}}(i) \geq 4$ are called columnar particles. Finally, two columnar particles are part of the same cluster, if they are neighbors.

## Stack rotation moves

To speed up the equilibration of Monte Carlo simulations, especially the ones with hard cut spheres and double hard cut spheres, we implemented Monte Carlo moves that are designed specifically to rotate short stacks. We select a particle randomly and define a stack by the particles with a center-to-center distance smaller than the $0.5D$. The nematic axis of this stack is determined in the usual way [1] and a random vector in the plane perpendicular to this axis is generated. The stack is rotated around this axis by ninety degrees. Finally, the move is accepted if no overlaps are generated and rejected otherwise. This move can easily be seen to obey detailed balance. Furthermore, the simulation is ergodic because regular rotation and translation moves are also performed. Although the acceptance ratio of these moves is tiny $10^{-6}$, the small number of moves that are accepted during the simulation do significantly speed up the simulation.

## Coexistence

We directly simulate two coexisting phases: a columnar phase and an isotropic or cubatic phase. The initial configurations of these simulations consist of two phases of interest in contact. A typical snapshot of a simulation after initial equilibration, during which the cubatic phase transforms into an isotropic fluid, is shown in Fig. 1(a). In Fig. 1(b), the nematic order parameters as obtained from such simulations for cut spheres and a range of pressures are shown. Clearly the cubatic phase transforms into the columnar phase

[*] Currently at HHU, Düsseldorf, Germany
[†] Currently at IQAC-CSIC, Barcelona, Spain

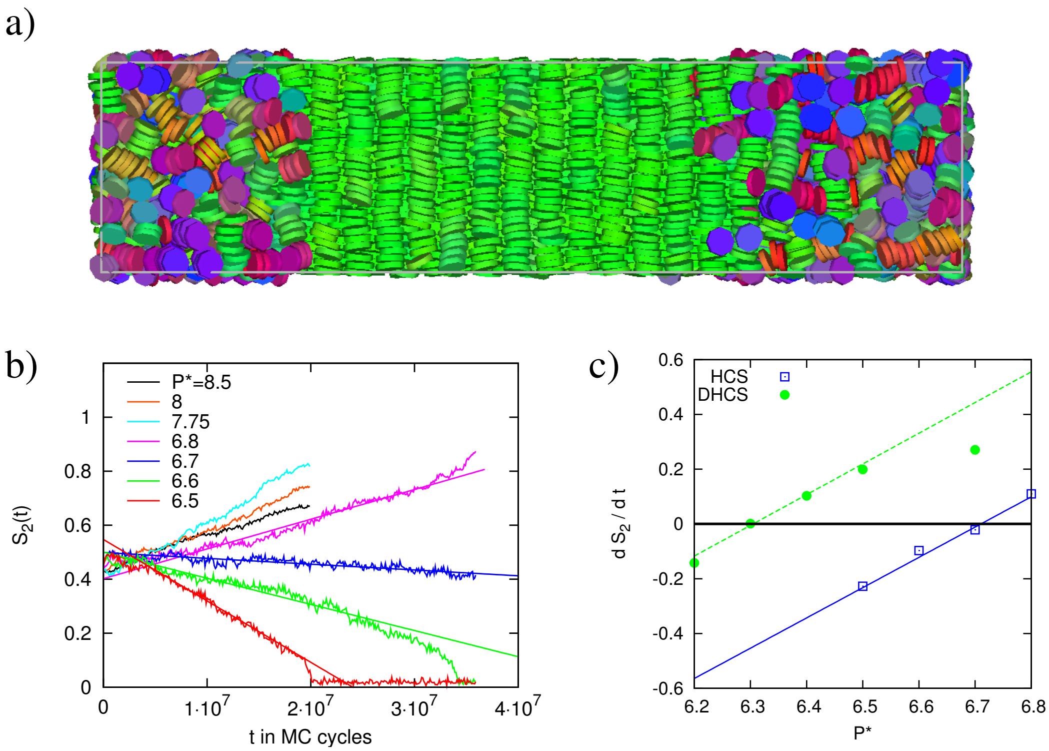


FIG. 1. (a) The initial configuration of each of the simulations in which we determine the pressure at coexistence between the isotropic phase and the columnar phase consists of a fluid phase and a columnar phase joined together in a single simulation box for cut spheres after equilibration at $P^* = 6.8$. (b) Nematic order parameter $S_2$ versus the number of MC cycles in $NPT$ simulations of cut spheres at pressures $P^* \equiv \beta P v_{\rm CS}$ as labeled. The straight lines are linear fits to the straigth sections of the curves. (c) The fits from (b) as a function of the pressure $P^*$ and the corresponding plot for double hard cut spheres. The straight lines are linear fits. The outlier for DHCS is too far from coexistence to fall on a straight line (see text) and is therefore not included in the fit.

for the pressures where the isotropic phase was stable $P^* \equiv \beta P v_{HCS} \geq 7.75$. This shows unambiguously that the cubatic phase is not stable for any of these densities.

Fits to the nematic order parameter [straight lines in Fig. 1(b)] near the coexistence can be used to determine the coexistence pressure [2]. This process is shown in Fig. 1(c). The slope of the linear fits to $S_2(t)$ is denoted $d\,S_2(t)\,/\,d\,t$. The coexistence pressure is the pressure for which $d\,S_2(t)\,/\,d\,t = 0$. The growth speed can be shown to be proportional to $D[\exp(\beta\Delta\mu) - 1]$ [3], where $\Delta\mu$ is the supersaturation (the chemical-potential difference between the two phases in contact) and $D$ is the self-diffusion constant. Near coexistence we use this to approximate $d\,S_2(t)\,/\,d\,t \simeq a\Delta\mu = a\int(1/\rho_I - 1/\rho_C)dP \simeq b\Delta P$, where $\rho_I$ and $\rho_C$ are the densities of the isotropic and columnar phases, respectively. Furthermore, we assume that the pressure difference $\Delta P$ is small enough that all properties of the two phases in the simulation box are approximately equal to those of the system at coexistence, such that $a$ and $b$ are approximately constant. In practice, we fit a linear function to $d\,S_2(t)\,/\,d\,t$ as a function of $P^*$ and calculate the pressure for which this straight line intersects with the line $d\,S_2(t)\,/\,d\,t = 0$ (the thick black line in Fig. 1). In Fig. 1(c), a point far from the coexistence is plotted to show that deviations from linearity are indeed a real possibility. This

| Shape $S$ | $d(S,\mathrm{Cyl})$ | $P^*$ | $\eta_I$ | $\eta_C$ | $\eta_{\rm cub}$ |
|---|---|---|---|---|---|
| DHCS | 0.00165836 | 6.304(7) | 0.4639(4) | 0.5336(3) | 0.495(5) |
| HCS | 0.00653491 | 6.710(8) | 0.4788(4) | 0.5502(3) | 0.505(5) |
| OHSC [4] | 0.02527792 | 8.276 | 0.5052 | 0.5705 | 0.57(1) |

TABLE I. The pressures and packing fractions at coexistence between the isotropic ($I$) and columnar ($C$) phases for HCS and DHCS from this work and for OHSC from Ref. [4]. Also shown is the Haussdorf distance $d(S,\mathrm{Cyl})$ between a cylinder (Cyl) and each of the three shapes $S$. Furthermore, the packing fraction $\eta_{\rm cub}$ at which the cubatic order increases suddenly on increase of the density is listed in the last column.

outlier is not included in the fit. The resulting coexistence data are listed in Tbl. I together with the data for the OHSC for reference.

# Difference between shapes

The difference between shapes as plotted in the phase diagram, Fig. 5 of the main text, is defined using the Hausdorff distance [5]. In order to define this distance on shape space, which is commonly used in (convex) geometry, we first define

$$d'(A,B) = \max_{\mathbf{x}\in A}\min_{\mathbf{y}\in B}|\mathbf{x}-\mathbf{y}| \tag{2}$$

where $A$ and $B$ are solid (compact) bodies. The Hausdorff distance is then defined by

$$d(A,B) = \max\{d'(A,B), d'(B,A)\}. \tag{3}$$

For solid (compact) bodies, it can easily be seen that, for the two points $\mathbf{x}$ and $\mathbf{y}$ at a local minimum–maximum in Eqn. (2), (i) $\mathbf{x}$ lies on the surface $\partial A$ of body $A$, while (ii) $\mathbf{y}$ lies on $\partial B$, (iii) $\mathbf{x}-\mathbf{y}$ is an outward normal to the surface of $A$ in $\mathbf{x}$ and (iv) $\mathbf{x}-\mathbf{y}$ is also an outward normal to the surface of $B$ in $\mathbf{y}$ (in the case of a cusp at one of the two points, $\mathbf{x}-\mathbf{y}$ has only to be normal to the path of the cusp at the point in question and point away from the body in question). Maximizing over all such pairs (of which there are only a few, if one takes into account the rotational symmetry) we can easily calculate the Hausdorff distance between a cylinder and an oblate hard spherocylinder, a hard cut sphere or a hard double cut sphere where all the shapes have the same aspect-ratio, volume and center-of-mass position and are co-aligned. The resulting values for the Hausdorff norm are listed in Tbl. I.

# Slow and collective dynamics

In Figs. 2(a) and (b), the mean squared displacement $\Delta r^2 \equiv \langle(\mathbf{r}_i(t)-\mathbf{r}_i(0))^2\rangle$ and the second order orientational correlation function $\Xi_2(t) = \left\langle \frac{3}{2}[\mathbf{u}_i(t)\cdot\mathbf{u}_i(0)]^2 - \frac{1}{2}\right\rangle$ are shown as obtained from event-driven MD simulations of OHSC at a packing fraction where the fluid is just thermodynamically stable, $\eta = 0.5$, and the packing fraction where nucleation is first observed, $\eta = 0.56$. We extract a time scale for translational dynamics by fitting a straight line $6D_l t$ to the long time behavior of the mean squared displacement, where $D_l$, the long time self diffusion constant, is the fitting parameter. The time scale is then $\tau_t = D_l^2/6D$. Furthermore, we fit a stretched exponential $\exp[(t/\tau_r)^{\epsilon_r}]$ to $\Xi_2(t)$. The resulting values are $\tau_t = 13.9$ and $\tau_r = 4.0$ for $\eta = 0.5$ and $\tau_t = 68.7$ and $\tau_r = 24.4$ for $\eta = 0.56$. The time scales for translation and rotation cannot be easily compared with each other due to the somewhat *ad hoc* definitions. However, we can see that both $\tau_t$ and $\tau_r$ increase by a factor of about 6 when increasing the density from $\eta = 0.5$ to $\eta = 0.56$. This behavior contrasts with that of ellipsoids with the same aspect ratio (short axis over long axis) 0.2, which shows a much faster increase of the rotational time scale with density than the translational time scale.

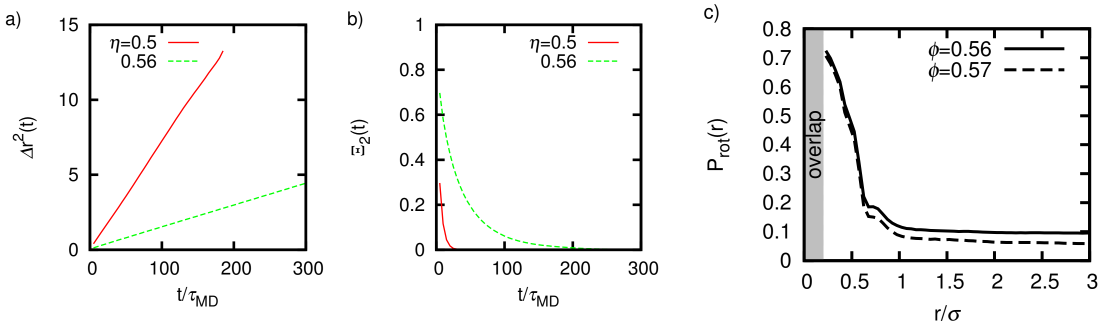


FIG. 2. (a) and (b) The long time behavior of the mean squared displacement $\Delta r^2(t)$ (a) and the second order orientational correlation function $\Xi_2(t)$ (b) as a function of time $t$ divided by $\tau_{\rm MD} = \sqrt{\beta m D^2}$. (c) The chance $P_{\rm rot}(r) = g_{\rm rot,rot}(r)/g_{\rm rot,all}(r)$, where $g_{s,s'}(r)$ is the radial distribution function that measures the distribution of particles of type $s'$ around particles of type $s$, and "all" denotes all particles, while "rot" denotes those particles that rotated more than 45 degrees between two snapshots that were taken at time intervals of $5\tau_{\rm MD}$.

The main mode of re-orientation is the collective rotation of the particle in a stack as can be seen in Fig. 2(c), which shows that, when a particle rotates more than 45 degrees, more than 60% of its neighbours with a center-of-mass distance smaller than $2L$ rotate along. This has consequences for the attachment to the columnar cluster, as shown in Fig. 3.

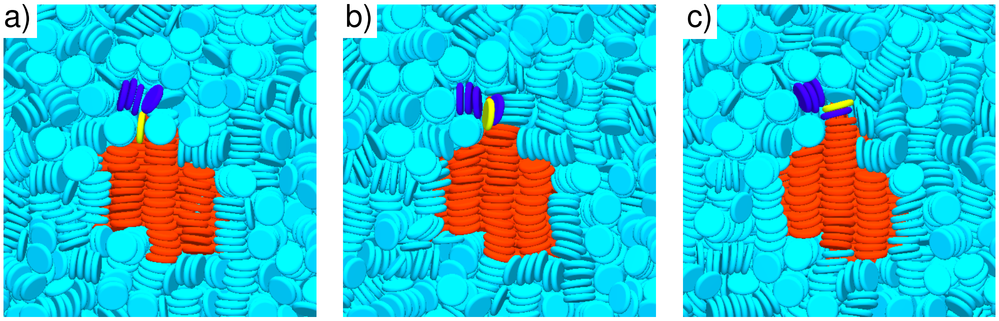


FIG. 3. (a) A particle (yellow) is misaligned with the columnar cluster (indicated by the red particles). (b) It slips in between the particles of a stack (dark blue). (c) Together with one of the particles of the stack, it rotates and becomes part of the columnar cluster.

[1] M. P. Allen, G. T. Evans, D. Frenkel, and B. M. Mulder, Advances in chemical physics **86**, 1 (1993).
[2] T. Zykova-Timan, J. Horbach, and K. Binder, J. Chem. Phys. **133**, 014705 (2010).
[3] S. Pronk and D. Frenkel, J. Chem. Phys. **110**, 4589 (1999).
[4] M. Marechal, A. Cuetos, B. Martínez-Haya, and M. Dijkstra, J. Chem. Phys. **134**, 094501 (2011).
[5] M. Moszyńska, *Selected topics in convex geometry* (Birkhäuser, Boston, 2006).
